# Supplementary material for: PDEInvBench: A Comprehensive Dataset and Design Space Exploration of Neural Networks for PDE Inverse Problems
Source: arXiv:2605.25353 source file (2026-05-26)
Supplement: Supplementary file 1 [file _s7_appendix_related_works.tex]

\section{Extended Related Works}
\label{sec:appendix-additional-related-works}

\paragraph{Inverse modeling using neural networks and Neural Operators.}

\wip{Our work fills in the gap of extensive evaluations on a variety of fluids datasets spanning different classes with complete measurements.}

There have been a number of non-NO methods proposed including~\citet{zhao_learning_2022} who develop an approach through learning a generative prior by pre-training both a coordinate network and a Graph Neural Network forward model. 
At test-time, they optimize a latent code to match sparse observations.
~\citet{pakravan_solving_2021} replace the decoder of an auto-encoder with numerical discretization schemes to recover PDE parameter \wip{fields}. \nc{what}
~\citet{goh_solving_2022} derive variational auto-encoders~\citep{kingma_auto-encoding_2013} from a divergence-based variational inference perspective to obtain uncertainty quantification for Bayesian inverse problems.
Our work contributes to this space by deriving general insights that apply across modeling frameworks.

\paragraph{Existing datasets and benchmarks.}

Several single-parameter datasets~\citep{lu_comprehensive_2022, bhan_pde_2024, toshev_lagrangebench_2024} and multi-parameter datasets~\citep{takamoto_pdebench_2022, gupta_towards_2022, hassan_bubbleml_2023} focused on fluid dynamics have been proposed.\nc{note to future self: pdearena has 117 bouancy values, pdebench has a handful (for the simpler systems they have more, bubbleml around 20, the well seems to have multiparam around 35 max, kohl benchmarking diffusion models 91 params}
However, the multi-parameter datasets, consisting of less than \nc{insert $n$} parameters, do not provide enough parameters to robustly evaluate inverse parameter estimation.
CFDBench~\citep{yining_cfdbench_2023} is likely the most amenable to evaluate inverse parameter estimation, but is insufficient to capture the wide range of physical systems our work covers. 
Meanwhile, existing benchmark studies have either focused exclusively on the PDE forward problem ~\citep{lu_comprehensive_2022}, or do not thoroughly study the inverse problem on multi-parameter datasets and across multiple design axes ~\citep{takamoto_pdebench_2022, hao_pinnacle_2023}, as in our work.

~\citep{liu_wavebench_2024} evaluate wave propagation problems but consists of a few number of physical parameters (< \nc{insert $n$}).
Multi-domain collections similarly vary in parameter richness: from single-parameter benchmarks~\citep{hao_pinnacle_2023, burark_codbench_2024} to those with modest multi-parameter support~\citep{ohana_well_2024, herde_poseidon_2024}. 
More specialized datasets include~\citep{trifonov_condiff_2025} for diffusion equations,~\citep{dulny_dynabench_2023} for low-resolution dynamics,~\citep{ren_superbench_2025} for super-resolution (all with fixed or limited parameters). 
~\citet{yu_climsim_2023} for climate science focused data, unsuitable for evaluating PDE parameter estimation performance.

Existing have given limited attention to inverse problems.
 performs extensive comparisons on forward problems without investigating NOs for inverse tasks. ~\citep{takamoto_pdebench_2022} explore the performance of FNO and UNet on inverse problems primarily by estimating initial conditions for trajectories using surrogate forward models trained on single-parameter datasets, but do not predict physical parameters or train on multi-parameter datasets. 
~\citep{hao_pinnacle_2023} evaluates inverse estimation of PDE coefficients for time-independent PDEs, but focuses mainly on comparing PINN variants rather than systematically exploring the design space for neural networks across diverse PDE systems. 
Our work fills these gap by performing extensive evaluation of FNO and other model architectures on the task of estimating the parameter coefficients of PDEs across a wide range of physical behavior.
